# Supplementary material for: A New Method for High-Resolution Dating of Radiocarbon Data: The Example of the First Three Centuries B.C
Source: arXiv:2502.20211 ancillary file (2025-02-27)
Supplement: Supplementary file 1 [file Anc01_Functionality_of_R_Simulate.pdf]

## Excursus on the Functionality of R\_Simulate in OxCal

For the method presented here, understanding the operation of the 'R\_Simulate' command is essential. In brief, when invoked, R\_Simulate generates a normally distributed random number based on a specified calendar date and a selectable standard deviation. By calibrating this number using the chosen calibration curve, a date is generated that one would expect for an object of a given age, taking into account the achievable accuracy (Bronk Ramsey 2001, 360).

The syntax of the command is as follows:

```
R_Simulate("Name", CalendarDate, StandardDeviation)
```

For example, the command R\_Simulate(-200,20) produces an uncalibrated radiocarbon age and a corresponding calibrated date range based on a calendar date of 200 BC and a measurement uncertainty of  $\pm 20$  years. In the present study, however, was omitted, as the randomly generated  $^{14}\text{C}$  age would otherwise not have been displayed. The provision of a name in the 'R\_Simulate' command was omitted, as including one would have prevented the randomly generated  $^{14}\text{C}$  age from being displayed.

The 'R\_Simulate' function incorporates several sources of statistical uncertainty, as illustrated by the following example calculations. Even when the nominal standard deviation is set to  $\pm 0$  years, method-inherent fluctuations can yield different radiocarbon ages. For instance, five identical executions of R\_Simulate(-200,0) result in four values that are very similar (2175.84 BP, 2175.56 BP, 2177.99 BP and 2174.73 BP), while a fifth computation produces a notably different radiocarbon age of 2195.82 BP (see **figure 1a** in the main article). This discrepancy arises because there is already a normally distributed spread about the expected value ( $\mu = 200 \text{ BC}$ ).

Bronk Ramsey (2009a) emphasises that “the measurement is made on the isotopic composition of the sample, not on the age of the sample”. This observation accounts for the sometimes broad dispersions, which are further amplified by the isotopic composition of the atmosphere as manifested in the calibration curve.

This dispersion is further increased when a standard deviation is specified: in one instance, five runs of R\_Simulate(-200,20) produced radiocarbon ages of 2225 BP, 2151 BP, 2227 BP, 2199 BP, and 2232 BP (see **figure 1b** in the main article). Moreover, the form of the calibration curve can further extend the dating range of the calibrated probability distribution. In the example provided, all five 95.4% ( $2\sigma$ ) intervals span well over 100 years, with the overall potential dating range extending from -382 calBP (for the 2232 BP measurement) to 78 calAD (for the 2225 BP measurement).

These examples illustrate the issue that uncertainties tend to accumulate, resulting in extremely wide time ranges. Consequently, for certain periods—such as the later Iron Age—the method must rely on supplementary information from stratigraphy or archaeological context, as well as on statistical approaches like Bayesian modelling, to yield any meaningful chronological insight.

Another aspect that may lead to confusion concerns the shape of the calibrated probability distribution along the x-axis. The varying amplitudes of these distributions might be misconstrued as representing the actual probabilities of the target calendar date. In reality, they merely indicate the intersections of the Gaussian bell curve with the calibration curve: the closer a point lies to the bell curve's mean, the higher the displayed probability on the x-axis. However, the calibrated probability distribution does not provide any information about where the target calendar date actually falls along the y-axis of the bell curve.

**Figure 1**, which displays the curve plots from the five *R\_Simulate* computations, clearly demonstrates that an event to be dated (in this case, 200 BC) can, in some instances due to an unfavourable shape of the calibration curve, fall significantly at the margins of the probability distributions. In three out of the five cases, the underlying calendar date of the measurement even lies outside the  $2\sigma$  (95.4%) range.

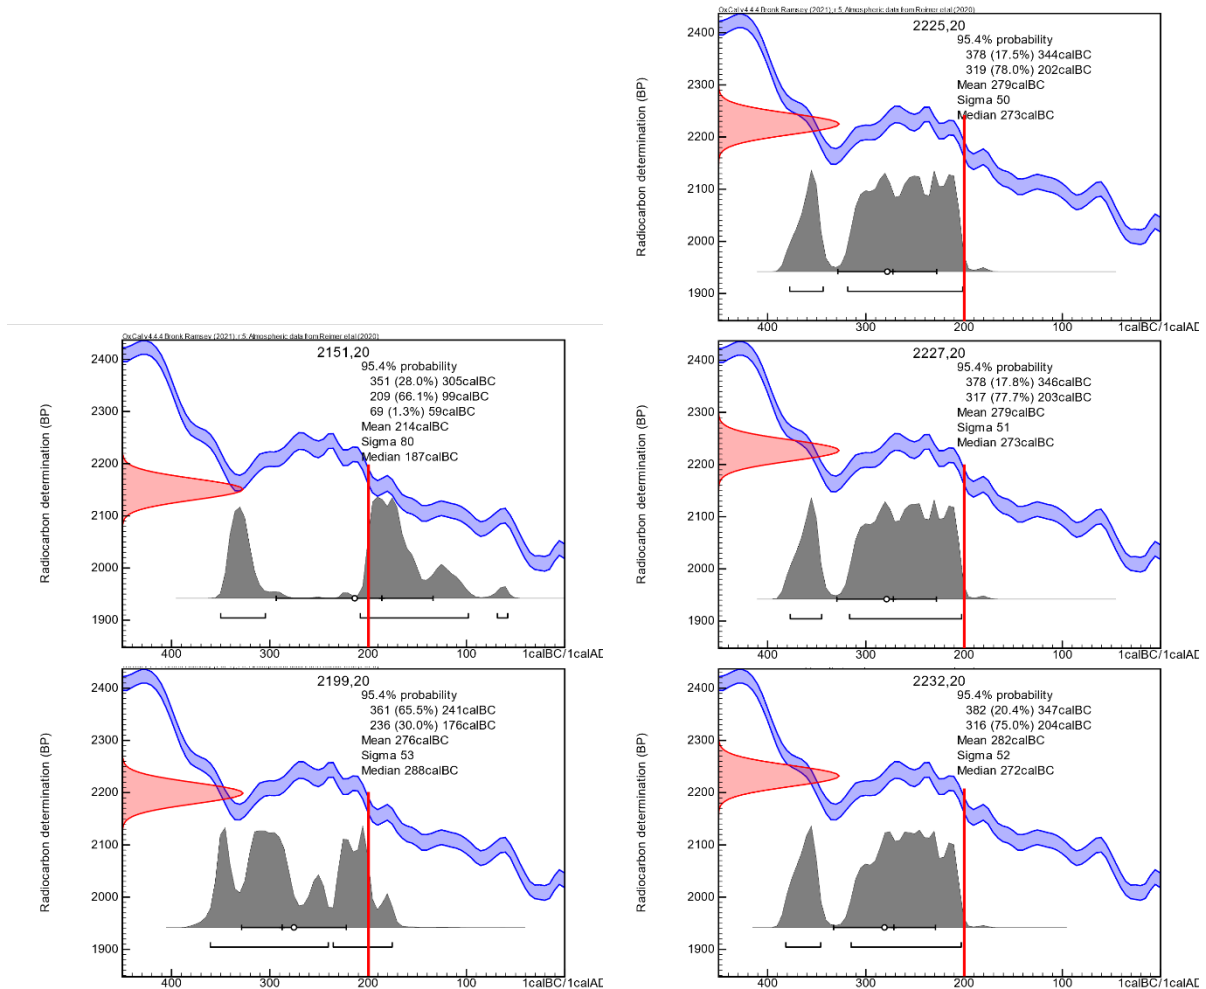

Figure 1. Curve plots for the five *R\_Simulate* computations (cf. fig. 1 in the main article). The position of the reference date on the x-axis is highlighted in red. A small white dot beneath the calibrated radiocarbon probability distribution denotes the arithmetic mean, while a small black cross adjacent to it indicates the median. The brackets below display the  $2\sigma$  range.

At the same time, it becomes apparent that the medians of the computations allow for a reasonably close approximation. The median of the five medians is 273, while the arithmetic mean of the values is 258.6—both of which are closer to the actual date than the shape of the curves might suggest. Moreover, the extent of the sigma interval does not appear to be an indicator of a deviating median. Notably, in our example the best approximation is provided by the median of the 2151 BP computation (corresponding to 187 calBC), despite a sigma of 80 years. The significance of the arithmetic means and medians for the estimation procedure presented herein will be discussed in further detail below.

The utility of multiple measurements is further illustrated by another *R\_Simulate* example. In this instance, three measurements were generated based on the year 37 BC with a standard deviation of  $\pm 20$  years (see **figure 2**).

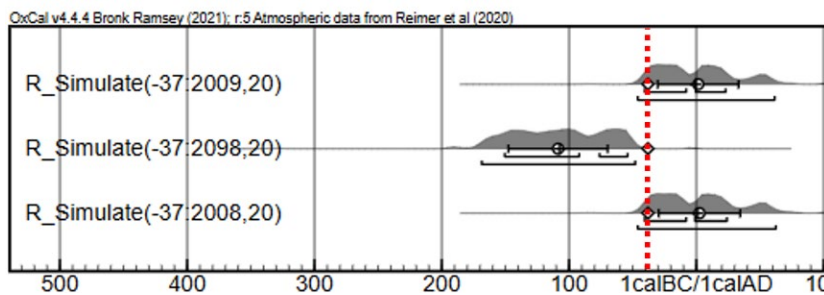

Figure 2. The three generated calibrated probability distributions. The position of the underlying calendar date (37 BC) is indicated in red.

In all three measurements, the underlying date is located at the extreme edge of the probability distributions. In one instance (2098 BP), it even falls outside the  $2\sigma$  (95.4%) range (as indicated by the lower bracket beneath the probability distributions). Owing to the shape of the calibration curve in this region, the resulting probability distributions are highly heterogeneous. Some uncalibrated radiocarbon ages—such as 2098 BP—produce pronounced outliers towards older dates, whereas radiocarbon ages of 2008 and 2009 BP yield the opposite effect, with the respective probability distributions suggesting a younger date.

Thus, the ‘R\_Simulate’ command can be employed to generate realistic simulations of the various uncertainties inherent in radiocarbon dating that give rise to the well-known dating ranges—albeit with the significant heuristic advantage of revealing the actual underlying date ‘behind the scenes’. This capability facilitates the development of strategies to improve dating accuracy. In particular, it becomes evident that multiple measurements of a single object can significantly narrow the dating range; here, not only is the arithmetic mean of the uncalibrated data beneficial, but more importantly, the calculation of the mean or median from the positions of the calibrated probability distributions. This is because the sometimes problematic shape of the calibration curve can have an amplifying effect, whereby even slight differences in radiocarbon ages—expected as a result of method-inherent fluctuations—can lead to markedly divergent probability distributions upon calibration.
