# Supplementary material for: A New Method for High-Resolution Dating of Radiocarbon Data: The Example of the First Three Centuries B.C
Source: arXiv:2502.20211 ancillary file (2025-02-27)

Overview of the histograms of the fine dating parameters for the reference table 5\_100\_0.

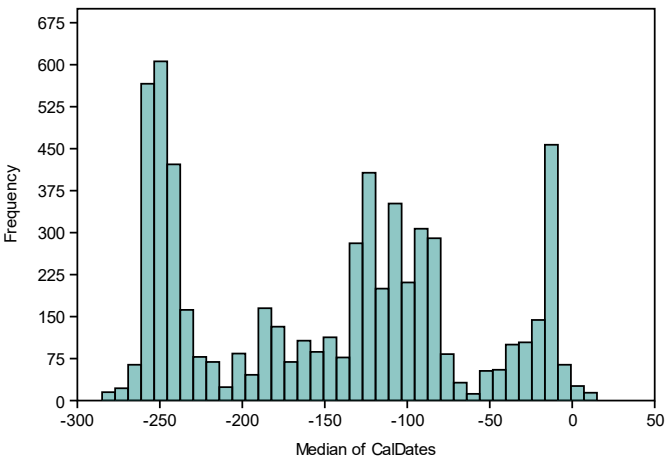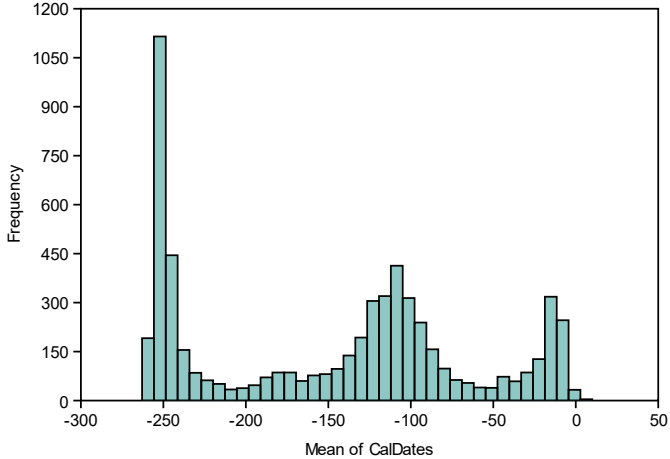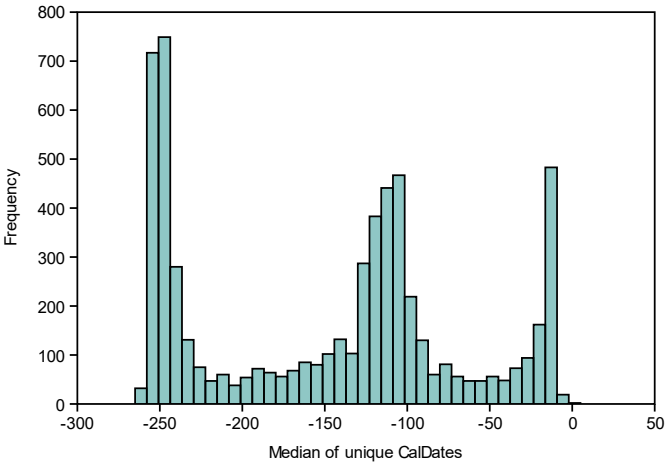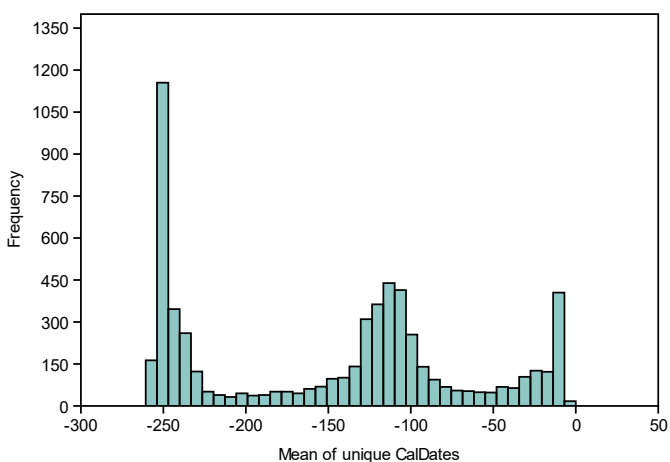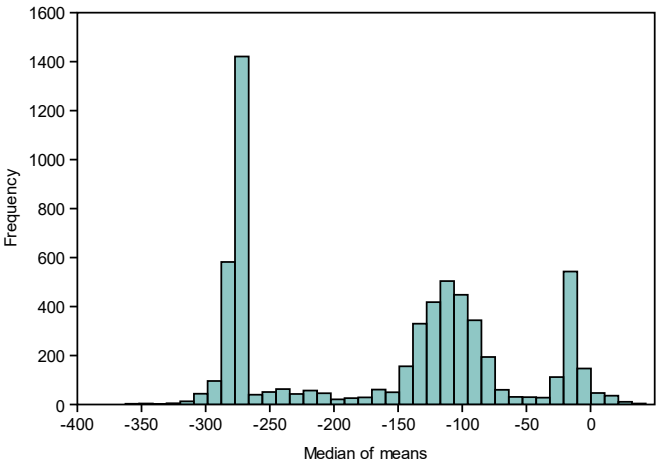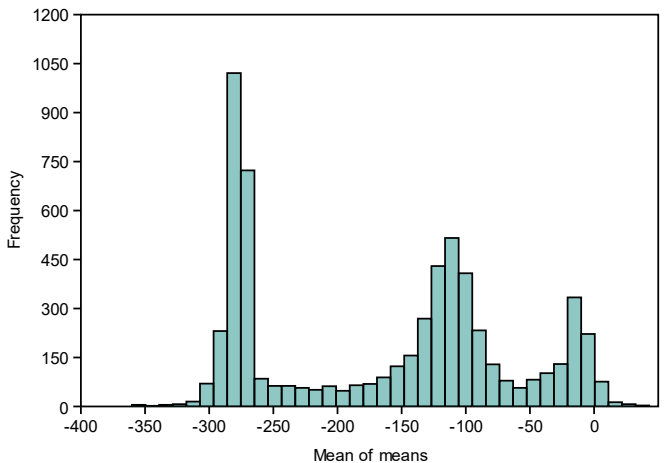

Overview of the histograms of the fine dating parameters for the reference table 5\_100\_0.

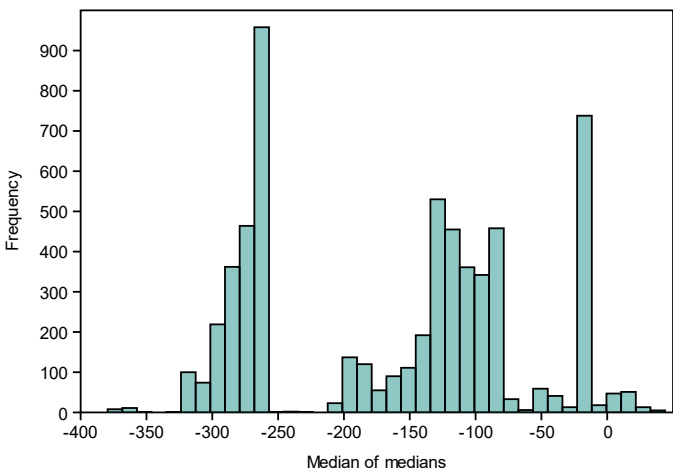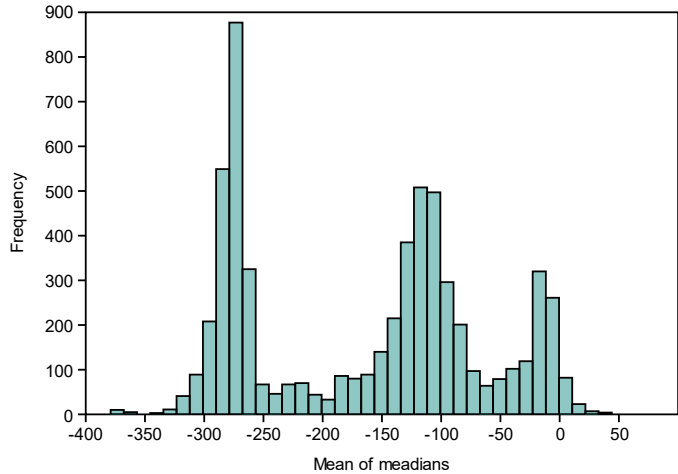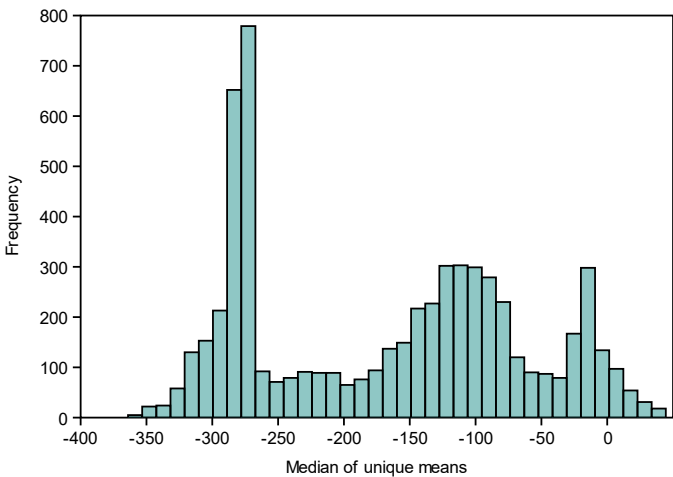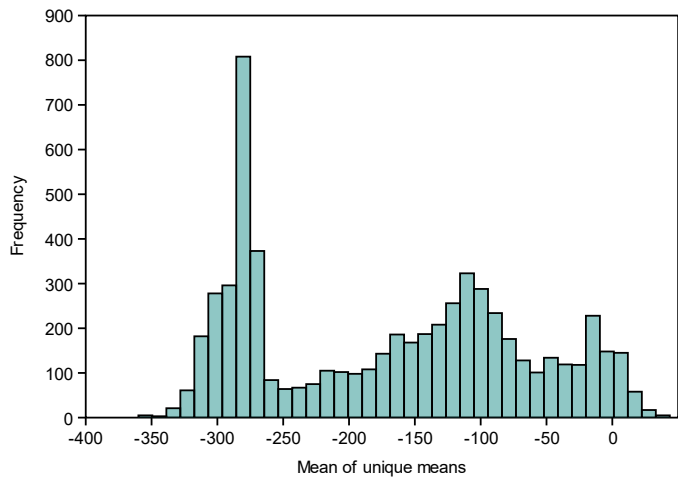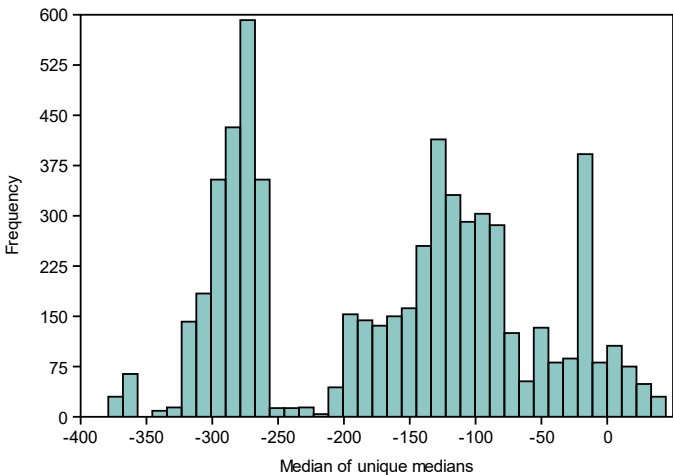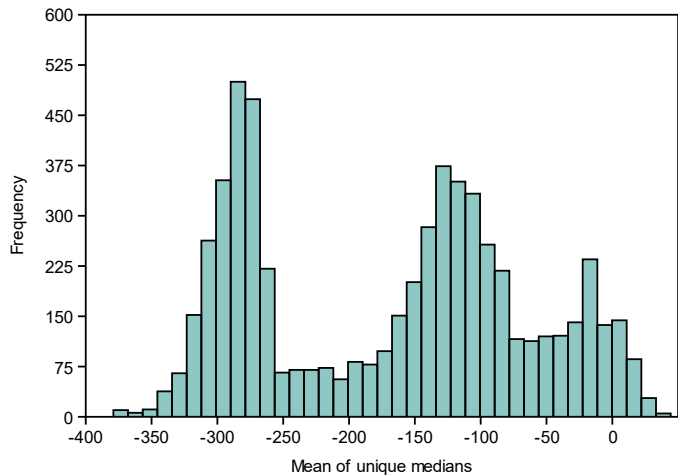

Supplement: Supplementary file 2 [file Anc12_Histograms_FineDating_5_100_0.pdf]
